# Supplementary material for: Estimating Excitonic Effects in the Absorption Spectra of Solids: Problems and Insight from a Guided Iteration Scheme
Source: arXiv:1412.0093 ancillary file (2015-03-26)
Supplement: Supplementary file 1 [file tddftrbo_supplement.pdf]

# Supplementary material for: "Estimating Excitonic Effects in the Absorption Spectra of Solids: Problems and Insight from a Guided Iteration Scheme"

Santiago Rigamonti,[1,2,*] Silvana Botti,[3,4,2] Valérie Veniard,[5,2]
Claudia Draxl,[1,2] Lucia Reining,[5,2,†] and Francesco Sottile[5,2]
[1] *Physics Department, Humboldt-Universität zu Berlin, Germany*
[2] *European Theoretical Spectroscopy Facility (ETSF)*
[3] *Institut Lumière Matière, UMR5306 Université Lyon 1-CNRS, Université de Lyon, F-69622 Villeurbanne Cedex, France*
[4] *Friedrich-Schiller Universität Jena, Institut für Festkörpertheorie und -optik, Max-Wien-Platz 1 07743 Jena*
[5] *Laboratoire des Solides Irradiés, École Polytechnique, CNRS, CEA-DSM, F-91128 Palaiseau, France*
(Dated: January 30, 2015)

## COMPUTATIONAL DETAILS

We have calculated the ground state for Si, LiF and Ar using density-functional theory [1] in the local-density approximation (LDA) [2]. For the results shown in the figures, we have used plane-waves basis sets and norm-conserving Troulliers-Martins pseudopotentials [3]. The pseudopotentials for LiF and Si were taken from the Abinit pseudopotential website [4]. The case of Argon turned out to be more delicate and required a separate treatment (the standard available pseudopotentials for Ar are ineffective in reproducing the all-electron results as obtained with the `exciting` code [5]). We generated the corresponding pseudopotential using the code Opium [6]: We have used the Perdew-Wang parametrization [7], the ionized filling suggested by Bachelet, Hamann, and Schlüter [8] ($3s^1 3p^{4.75} 3d^{0.25}$), and a cutoff radius of 1.5 Bohr radii for the three s, p, d components. In Si, the energy cutoff is 20 Hartree, while it is 40 Hartree for LiF and 70 Hartree for Ar. For the spectra we used a grid of 256 inequivalent (out-of-symmetry [9, 10]) k-points for LiF and Si, and 2048 k-points for Ar. The ground state for all systems was obtained with a Monkhorst-Pack grid of 256 shifted k-points in the whole Brillouin zone [11]. Experimental lattice constants were used for the calculations: 10.22 a.u. for Si, 7.59 a.u. for LiF and 9.932 a.u. for Ar. We used $N_G = 59$ for Si, 169 for LiF, and 181 for Ar in order to obtain well converged spectra with respect to local-field effects. We have corrected the electronic bandstructure of the three materials using a rigid shift of the conduction bands to mimic quasiparticle energies. These shifts are 0.8 eV, 5.27 eV, and 5.84 eV for Si, LiF, and Ar, respectively, in order to simulate the corresponding experimental photoemission band-gap $E_g$ at the $\Gamma$ point. Experimental values are available in Refs. [12, 13] for Si ($E_g^{\mathrm{Si}} \approx$ 3.4 eV, corresponding to the $E_0'$ transition at $\Gamma$), [14] for LiF ($E_g^{\mathrm{LiF}} \approx 14.2$ eV), and [15] for Ar ($E_g^{\mathrm{Ar}} \approx 14.15$ eV). Bethe Salpeter equation calculations (as obtained with the EXC code [16], not shown) and QP-RPA spectra (as well as the long-range kernel for Si, not shown) are converged with 7 bands; however BO and RBO calculations require a higher number of bands, namely 8 for Si, 20 for Ar and 30 for LiF. An overall Lorentzian broadening of 0.1 eV has been applied. Ground state calculations have been performed with the Abinit code [17], while all RPA, BO, and RBO calculations have been obtained with the DP code [18]. All the results for the BO, RBO and QP-RPA kernels have also been obtained with the full-potential all-electron code `exciting` [5], and are consistent with the results shown in this paper. Besides, a family of matrix kernels obtained according to the guided iteration idea has been developed and studied in detail with `exciting` [19].

## QUASIPARTICLE GAP

For a correct interpretation of the calculated spectra it is crucial to be clear on the quasiparticle gap that enters the calculation of $\chi^0$. In Fig. 1 we have put the digitalized data for LiF from Ref. [20] for both the RPA calculation (upper panel, dashed orange line) and the BO result (lower panel, dashed orange line). The onset of the RPA spectrum should coincide with the quasiparticle, i.e., the photoemission, gap, here represented by the vertical green line at 14.2 eV. However, the onset is at a much lower energy. By applying a shift of 1.2 eV towards higher energy, the RPA of [20] is superposed with our QP-RPA result, whose onset is at the quasiparticle gap (compare the dash-dot violet line with the full red line, in the upper panel). This indicates that the calculation in [20] was made using a quasiparticle gap about 1.2 eV smaller than the experimental one. A rigid shift in the RPA spectrum essentially translates into a rigid shift of the final spectrum including the electron-hole interaction. Indeed, if we shift the BO result of Ref. [20] (dashed orange line, lower panel) rigidly by 1.2 eV to higher energy, the result (dashed-dot violet line) falls on top of our BO calculation (full red line, lower panel). This demonstrates that our calculations and the calculations of [20] obtain the same, very small, exciton binding energies, and that the agreement with experiment is only apparent due to the too small quasiparticle gap used in

[20].

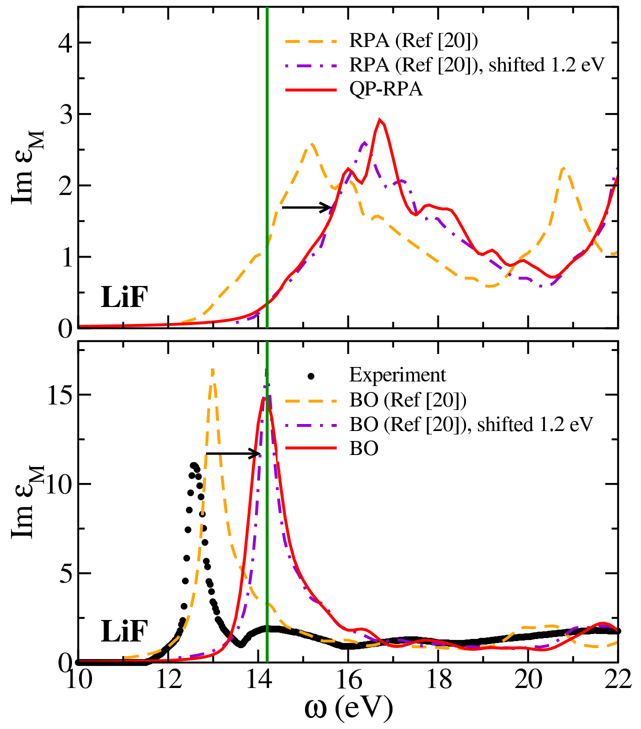


FIG. 1. (Color online) Imaginary part of the macroscopic dielectric function of LiF. Upper panel: red solid line: QP-RPA, present result; dashed orange line: RPA, result of Ref. [20]; dashed-dot violet line, RPA result of Ref. [20], shifted by 1.2 eV. Lower panel: circles: experiment [21]; red solid line: BO, present result; dashed orange line: BO from Ref. [20]; dashed-dot violet line: BO from Ref. [20] shifted by 1.2 eV. The vertical green solid line represents the photoemission band-gap (14.2 eV).

* srigamonti@physik.hu-berlin.de
† lucia.reining@polytechnique.edu

[1] P. Hohenberg and W. Kohn, Phys. Rev. **136**, B864 (1964).
[2] W. Kohn and L. J. Sham, Phys. Rev. **140**, A1133 (1965).
[3] N. Troullier and J. L. Martins, Phys. Rev. B **43**, 1993 (1991).
[4] Pseudopotentials for the ABINIT code: `http://www.abinit.org/downloads/psp-links/psp-links/lda_tm`.
[5] A. Gulans, S. Kontur, C. Meisenbichler, D. Nabok, P. Pavone, S. Rigamonti, S. Sagmeister, U. Werner, and C. Draxl, Journal of Physics: Condensed Matter **26**, 363202 (2014).
[6] OPIUM pseudopotential generation program: `http://opium.sourceforge.net/`.
[7] J. P. Perdew and Y. Wang, Phys. Rev. B **33**, 8800 (1986).
[8] G. B. Bachelet, D. R. .Hamann, and M. Schlüter, Phys. Rev. B **26**, 4199 (1982).
[9] J. A. Soininen and E. L. Shirley, Phys. Rev. B **61**, 16423 (2000).
[10] F. Sottile, V. Olevano, and L. Reining, Phys. Rev. Lett. **91**, 056402 (2003).
[11] H. J. Monkhorst and J. D. Pack, Phys. Rev. B **13**, 5188 (1976).
[12] K. H. Hellwege and O. Madelung, eds., “Numerical data and functional relationships in science and technology,” (Springer, Berlin, 1982).
[13] P. Lautenschlager, M. Garriga, L. Vina, and M. Cardona, Phys. Rev. B **36**, 4821 (1987).
[14] M. Piacentini, D. W. Lynch, and C. G. Olson, Phys. Rev. B **13**, 5530 (1976).
[15] M. Runne and G. Zimmerer, Nuclear Instruments and Methods in Physics Research Section B: Beam Interactions with Materials and Atoms **101**, 156 (1995).
[16] L. Reining, V. Olevano, F. Sottile, S. Albrecht, and G. Onida, “The exc code,” Unpublished.
[17] X. Gonze, J.-M. Beuken, R. Caracas, F. Detraux, M. Fuchs, G.-M. Rignanese, L. Sindic, M. Verstraete, G. Zerah, F. Jollet, M. Torrent, A. Roy, M. Mikami, P. Ghosez, J.-Y. Raty, and D. Allan, Computational Materials Science **25**, 478 (2002).
[18] V. Olevano, L. Reining, and F. Sottile, “The dp code,” Unpublished.
[19] S. Rigamonti, S. Botti, V. Véniard, C. Draxl, L. Reining, and F. Sottile, In Preparation.
[20] S. Sharma, J. K. Dewhurst, A. Sanna, and E. K. U. Gross, Phys. Rev. Lett. **107**, 186401 (2011).
[21] D. M. Roessler and W. C. Walker, J. Opt. Soc. Am. **57**, 835 (1967).
